# Supplementary material for: Depth-dependent resistance of granular media to vertical penetration
Source: arXiv:1307.4638 source file (2013-09-16)
Supplement: Supplementary file 1 [file Supplement.pdf]

# Supplemental Material for "Depth-dependent resistance of granular media to vertical penetration" Part I. Theory

T. A. Brzinski III, P. Mayor, and D. J. Durian
University of Pennsylvania, Department of Physics & Astronomy

Here we supply theoretical details used in the main text. The first section is on models for the rate-independent granular friction force, including the effect of a sub-fluidizing upflow of air. The second and third sections are on the resulting total force on objects of various geometries moving downward or horizontally, respectively. The fourth section is on solutions of Newton's second law for impact dynamics, based on rate-independent friction plus an inertial drag that scales as speed-squared.

## 1 Models for the friction force

The rate-independent granular friction force on a unit area $\mathrm{d}A$ of a projectile could, in principle, act in some combination of normal $\hat{\mathbf{n}}$ and tangential $\hat{\mathbf{t}}$ directions. In any case the force must be proportional to a friction coefficient, $\mu = \tan^{-1}\theta_{\mathrm{repose}}$, and the hydrostatic pressure $\rho g z$, where $\rho$ is the bulk density of the granular medium, $g = 980$ cm/s$^2$, and $z$ is the depth of the area element, measured downward in the direction of gravity. The two extreme possibilities are thus

$$\mathrm{d}\mathbf{F} = \alpha_n\, \mu\rho g z\, \mathrm{d}A\, \hat{\mathbf{n}}, \tag{1}$$

$$\mathrm{d}\mathbf{F} = \alpha_t\, \mu\rho g z\, \mathrm{d}A\, \hat{\mathbf{t}}. \tag{2}$$

Here $\alpha_n$ and $\alpha_t$ are dimensionless constants; their values ought to be the same in all experiments, while only the value of $\mu\rho g$ reflects the nature of the materials.

When there is an upflow of air through the granular packing, the hydrostatic pressure and the responsible grain-grain contact forces decrease because air drag helps support the weight of the grains. Since the speed of the air flow is proportional to the imposed pressure drop, the hydrostatic pressure gradient in Eqs. (1-2) thus modifies to

$$\rho g \rightarrow \rho g(1 - U/U_c). \tag{3}$$

Here $U$ is the superficial air speed, equal to the volume flow rate per cross sectional area, and $U_c$ is the fluidization speed at which gravity and air drag are balanced and

the grain-grain contact forces all vanish. This holds for $U \leq U_c$, the condition for all experiments reported in the main text[†].

## 2 Friction on *downward*-moving objects

For any symmetrical object that moves downward through the granular medium, the vector sum of the friction forces on all surface area elements will point upward whether the force acts normal or tangential to the surface. Starting from Eqs. (1-2), we now carry out the integration appropriate for objects of various shapes. In all cases we assume that the top free surface of the granular medium remains horizontal and unperturbed.

### 2.1 Vertical cylinder

Perhaps the simplest geometry is a vertically-oriented right cylinder with radius $R$ and with total length greater than the distance $z$ of bottom circular face below the top free surface of the granular medium. If the granular friction acts normal to the surface, then the upward force is entirely due to the bottom face and hence is $\alpha_n \mu \rho g z$ times $\pi R^2$. But if the granular friction force acts tangential to the surface, then the upward force is entirely due to action along the vertical side of the cylinder. Specifically the upward force on a ring at depth $z'$ to $z' + \mathrm{d}z'$ is $\alpha_t \mu \rho g z'$ times area $\mathrm{d}A = 2\pi R \mathrm{d}z'$, integrated over $0 < z' < z$. The final results for the two cases are

$$F = \pi \alpha_n \ \mu \rho g R^2 z, \quad (4)$$

$$F = \pi \alpha_t \ \mu \rho g R z^2. \quad (5)$$

Note that the depth-dependence is linear for the former but quadratic for the latter, and hence can be distinguished by measurement.

### 2.2 Cone

For a right circular cone with opening angle $2\phi$, with apex at distance $z$ below the top free surface, the magnitude of the total upward friction force can be found by integrating over rings at distance $s$ from the apex. Since $s$ is measured along the

[†]For $U > U_c$ the grains are fluidized and the grain-grain contact forces vanish. The pressure drop across the sample then pegs at the total weight per area of the sample, and excess gas escapes in the form of bubbles.

surface of the cone, the ring at depth $(z - s\cos\phi)$ has radius $s\sin\theta$ and surface area $\mathrm{d}A = 2\pi(s\sin\theta)\mathrm{d}s$. The maximum value of $s$ is $z/\cos\theta$. If the friction force acts normal to the surface, then the integral for the total vertical force is

$$F = \int_0^{z/\cos\theta} \alpha_n\ \mu\rho g(z - s\cos\phi)\sin\theta\ (2\pi s\sin\theta\mathrm{d}s). \tag{6}$$

Note that a factor of $\sin\theta$ is inserted between the depth and the $\mathrm{d}A$ terms in order to give the vertical component. If the friction force acts tangential to the surface, then a $\cos\theta$ factor is required instead. Carrying out the integration for the two cases gives

$$F = \frac{\pi}{3}\alpha_n\ \mu\rho g(\tan\phi)^2 z^3, \tag{7}$$
$$F = \frac{\pi}{3}\alpha_t\ \mu\rho g(\tan\phi) z^3. \tag{8}$$

This assumes that the cone is tall enough to extend above the medium. In both cases the net friction force scales as $z^3$, and the only difference is in the power of the $\tan\phi$ factor. For the normal case, note that the force is $\alpha_n\mu/3$ times the pressure $\rho g z$ at the tip times the cross-sectional area $\pi(z\tan\phi)^2$ of the cone at the top free surface.

## 2.3 Cylinder with conical tip

This geometry is identical to a cone if the depth $z$ of the tip is less than $R\cot\phi$ below the top free surface of the medium, where $R$ is the radius of the cylinder and $2\phi$ is the opening angle of the conical tip. For greater depths, the force on the tip is calculated by an alteration of Eq. (6) so that the upper integration limit is $s_{max} = R/\sin\phi$. The force on the side of cylinder is zero for the normal case, and is given by Eq. (5) with $z \to z - R\cot\phi$ for the tangential case. Altogether, for $z > R\cot\phi$, the total friction force acting on a cylinder with a conical tip is computed to be

$$F = \pi\alpha_n\ \mu\rho g R^2\left(z - \frac{2}{3}R\cot\phi\right), \tag{9}$$
$$F = \pi\alpha_t\ \mu\rho g R\left[z^2 - R\cot\phi\left(z - \frac{1}{3}R\cot\phi\right)\right]. \tag{10}$$

As a check, note that at $z = R\cot\phi$ equations (7-10) all reduce to $(\pi/3)\alpha\mu\rho g R^3$ times a factor of $(\cot\phi)$ for the normal case, or times $(\cot\phi)^2$ for the tangential case.

## 2.4 Sphere

For a sphere, separate cases must be considered depending on whether the depth $z$ of the bottom of the sphere is less than or greater than the radius $R$. For the latter case, we assume that the friction force acts only on the lower hemisphere. As demonstrated

for the cone geometry, integrals may be set up over constant-depth area elements. If the action is normal to the surface, then the resulting total upward friction force is

$$F = \pi\alpha_n\mu\rho g \begin{cases} (R - z/3)z^2 & z < R, \\ (z - R/3)R^2 & z > R. \end{cases} \tag{11}$$

At great depths, note that the result is the same as for a cylinder but translated by $R/3$. On the other hand, if the action is tangential to the surface, then the total upward friction force is

$$F = \frac{\pi}{3}\alpha_t\mu\rho g R^2 \begin{cases} \sqrt{(2 - \frac{z}{R})\frac{z}{R}}(3R - 2z + z^2/R) - 3R(1 - \frac{z}{R})\cos^{-1}(1 - \frac{z}{R}) & z < R, \\ \frac{1}{2}\left[3\pi z - (3\pi - 4)R\right] & z > R. \end{cases} \tag{12}$$

This is qualitatively similar to Eq. (11). In both cases, for $z < R$ the force grows from zero as depth to a power greater than one. And for both cases, for $z > R$ the force is linear in projected area $\pi R^2$ times depth $z$. One notable difference in form is that the linear depth dependence extrapolates to zero force at $z = R/3$ for the normal case but at $z = [1 - 4/(3\pi)]R \approx 0.58R$ for the tangential case.

## 2.5 Horizontal cylinder

For a horizontal cylinder of radius $R$ and length $L$, moving downward, separate cases must be considered for depths $z$ less than or greater than $R$ just as for spheres. Also as for spheres, we assume that the friction force acts only on the lower half of the projectile. If friction acts normal to the surface, then the net upward force is

$$F = \alpha_n\mu\rho g L R \begin{cases} \sqrt{(2 - \frac{z}{R})\frac{z}{R}}(z - R) + R\cos^{-1}(1 - \frac{z}{R}) & z < R, \\ 2z - (2 - \pi/2)R & z > R. \end{cases} \tag{13}$$

If friction act tangential to the surface, then the net upward force is

$$F = \alpha_t\mu\rho g L \begin{cases} z^2 & z < R, \\ R(2z - R) & z > R. \end{cases} \tag{14}$$

## 2.6 Summary of results used in main text

By experiment, we find that the quasi-static stopping force acts *normal* to the surface of the intruding object. The relevant predictions found above are thus

$$\frac{F}{\pi\alpha_n\mu\rho g} = \begin{cases} R^2 z & \text{cylinder}, \\ \tan^2\phi\ z^3/3 & \text{cone}, \\ (R - z/3)z^2 & \text{sphere}, z \le R, \\ (z - R/3)R^2 & \text{sphere}, z \ge R. \end{cases} \tag{15}$$

# 3 Friction on *horizontally*-moving objects

## 3.1 Horizontal cylinder

For a horizontal cylinder of radius $R$, diameter $D = 2R$, length $L$, axis at depth $z > R$ below the top free surface, and moving pependicular to the axis, the total friction force points opposite to the velocity and is computed as follows. If the action is normal to the surface, the force is

$$\begin{aligned} F &= \int_{-\pi/2}^{\pi/2} \alpha_n \mu\rho g(z - R\sin\theta)\cos\theta \ (LR\mathrm{d}\theta). \\ &= \alpha_n \mu\rho g L D z. \end{aligned} \tag{16}$$

The first term in brackets is the depth of the area element $LR\mathrm{d}\theta$, and the $\cos\theta$ term gives the horizontal projection of the force. If the action is tangential to the surface, then the force is

$$\begin{aligned} F &= \int_{-\pi/2}^{\pi/2} \alpha_t \mu\rho g(z - R\sin\theta)|\sin\theta| \ (LR\mathrm{d}\theta), \\ &= \alpha_t \mu\rho g L D z. \end{aligned} \tag{17}$$

Here the $|\sin\theta|$ term gives the horizontal projection of the force. Note that in both cases the integrals evaluate to $\alpha\mu\rho g$ times depth times projected area $LD$, with the same numerical prefactor of one.

The torque on a horizontal cylinder rotated around a vertical axis midway along its length can be computed from the above force law. According to Eqs. (16-17), the differential force on the element of the cylinder between $r$ and $r + \mathrm{d}r$ from the rotation axis is $\mathrm{d}F = \alpha\mu\rho g(D\mathrm{d}r)z$. This assumes that the cylinder is thin, $D \ll r$. The total torque on the cylinder is then

$$\begin{aligned} \tau &= 2\int_0^{L/2} r[\alpha\mu\rho g z D\mathrm{d}r], \\ &= \frac{1}{4}\alpha\mu\rho D L^2 z. \end{aligned} \tag{18}$$

The final predicted torque expression is the same as that quoted in the 2010 article by Brzinski and Durian [1]. There, torque measurements for various cylinders, immersed to various depths into different granular media subjected to a range of sub-fluidizing upward airflows, were found to follow the form of Eq. (18) and to give a numerical prefactor of $\alpha = 15 \pm 2$.

## 3.2 Vertical cylinder

For a vertical cylinder of radius $R$, taller than the depth $z$ of its bottom end, and moving horizontally, the drag force is computed as follows. If the action is normal to

the surface, the force is

$$\begin{aligned} F &= \int_0^z \int_{-\pi/2}^{\pi/2} \alpha_n \mu \rho g (z') \cos\theta \ (R\mathrm{d}\theta \mathrm{d}z'). \\ &= \alpha_n \mu \rho g R z^2. \end{aligned} \tag{19}$$

Note that the first term in brackets is the depth of the area element $R\mathrm{d}\theta\mathrm{d}z'$, and that the $\cos\theta$ term gives the horizontal projection of the force. This assumes that there is no force on the back half of the cylinder. If the action is tangential to the surface, the force is similarly

$$\begin{aligned} F &= \int_0^z \int_{-\pi/2}^{\pi/2} \alpha_n \mu \rho g (z') |\sin\theta| \ (R\mathrm{d}\theta \mathrm{d}z'). \\ &= \alpha_t \mu \rho g R z^2. \end{aligned} \tag{20}$$

Here $|\sin\theta|$ gives the horizontal projection of the force. Note that the force is $\alpha\mu\rho g$ times projected area $2Rz$ times average depth $z/2$, whether the action is normal or tangential. This geometry corresponds to experiments where the force is measured on a rod plunged into a rotating bucket of grains [2, 3, 4]. In the most recent of these articles [4], Costantino *et al.* report measurements for various diameter rods plunged to various depths into different granular media, where gravity was effectively tuned by submerging the medium with fluids of various densities. The data were found to collapse according to the forms of Eqs. (19-20) and to give a value of $\alpha = 20 \pm 6$, if we assume a typical friction coefficient of $\mu = \tan^{-1}(24^\circ)$.

## 3.3 Sphere

For a sphere of radius $R$ buried so that its center is at depth $z > R$ below the top free surface, and moving horizontally, the drag force for the two cases is computed to be

$$F = \pi \alpha_n \mu \rho g R^2 z, \tag{21}$$

$$F = \frac{\pi}{2} \alpha_t \mu \rho g R^2 z. \tag{22}$$

As for a horizontally-moving cylinder, as indeed for any symmetric object, the force is $\alpha_n \mu \rho g z$ times projected area if the force acts normal to the surface elements. If the force acts tangential to the surface elements, the total force is proportional to $\alpha_t \mu \rho g z$ times projected area but now with a numerical prefactor of 1/2.

# 4 Impact dynamics and penetration depth

In this section we compute the dynamics of a projectile of mass $m$ due to gravity, $mg$, a depth-dependent but rate-independent friction force $F(z)$, and a speed-dependent but depth-independent inertial drag force[‡] $mv^2/d_1$. Measuring the depth $z$ downward in the direction of gravity, so that the velocity $v = \mathrm{d}z/\mathrm{d}t$ is positive for downward motion, the equation of motion is then [5]

$$ma = \frac{\mathrm{d}K}{\mathrm{d}z} = mg - F(z) - mv^2/d_1, \tag{23}$$

where $K = mv^2/2$ is the kinetic energy of the projectile and $d_1$ has units of length. As demonstrated in Ref. [6], this can be solved for speed vs depth by multiplying the equation of motion by $\exp(2z/d_1)$, separating variables, and integrating:

$$Ke^{2z/d_1} - K_o = \int_0^z \left[mg - F(z')\right] e^{2z'/d_1}\mathrm{d}z'. \tag{24}$$

Here $K = mv^2/2$ represents the kinetic energy when the projectile is at depth $z$, and $K_o = m{v_o}^2/2$ represents the kinetic at the initiation of impact at depth $z = 0$ and speed $v_o$. By inspection, this can be differentiated with respect to $z$ to recover the equation of motion. For any friction force, $F(z)$, the right-hand size of Eq. (24) is to be evaluated and the speed is to be isolated as a function of depth.

For several of the projectile shapes considered above, the friction force increases with depth as

$$F(z) = kz^n, \tag{25}$$

where $n$ is a positive number and $k$ has units of force/length$^n$. Inserting this force into Eq. (24) and integrating gives speed-squared versus depth as

$$v^2 = \left[{v_o}^2 + \beta\frac{k{d_1}^{n+1}}{m}\right]e^{-2z/d_1} + gd_1\left(1 - e^{-2z/d_1}\right), \tag{26}$$

$$\beta = \left(-\frac{1}{2}\right)^n \Gamma(n+1, 0, -2z/d_1), \tag{27}$$

where $\Gamma(a, x_0, x_1)$ is the generalized incomplete gamma function. Note that $\beta$ is dimensionless and $k{d_1}^{n+1} = F(d_1)d_1$ has units of energy, so that dividing by $m$ gives a quantity with units of speed-squared. For the three main cases of interest, the $\beta$ term simplifies to

$$\beta = \frac{1}{2}\begin{cases} -1 + \left(1 - \frac{2z}{d_1}\right)e^{2z/d_1} & n = 1, \\ 1 - \left(1 - \frac{2z}{d_1} + \frac{2z^2}{{d_1}^2}\right)e^{2z/d_1} & n = 2, \\ -\frac{3}{2} + \frac{3}{2}\left(1 - \frac{2z}{d_1} + \frac{2z^2}{{d_1}^2} + \frac{4z^3}{3{d_1}^3}\right)e^{2z/d_1} & n = 3. \end{cases} \tag{28}$$

[‡]This comes from transfer of momentum to the medium. For fluid systems, inertial drag is often written as $\frac{1}{2}C\rho v^2 A$ where $C$ is a dimensionless coefficient, $\rho$ is the density of the medium, and $A$ is cross-sectional area of the projectile. However, expressions are simpler in terms of $d_1$ rather than $C$.

To find the penetration depth $d$ where a projectile comes to rest, Eqs. (26-27) are to be solved for the depth at which the velocity vanishes. In general this must be done numerically, but for the special case $n = 1$ the penetration depth may be found in closed form:

$$d = \frac{mg}{k} + \frac{d_1}{2}\left\{1 + W\left[\left(\frac{2m{v_0}^2}{k{d_1}^2} - \frac{2mg}{kd_1} - 1\right)e^{-\frac{2mg}{kd_1}-1}\right]\right\}, \tag{29}$$

where $W(x)$ is the product-log function, also known as the Lambert $W$-function, which is the inverse of $f(W) = W\exp(W)$.

Next we consider the case of a sphere that penetrates to a depth less than its radius, and a granular friction that acts normal to the surface. Then the force law is Eq. (11). This may be integrated in Eq. (24), which gives speed versus depth as

$$\begin{aligned} v^2 &= {v_o}^2 e^{-2z/d_1} + \left[gd_1 - \frac{\pi\alpha_n\mu\rho g}{4m}{d_1}^3(d_1+2R)\right]\left(1-e^{-2z/d_1}\right) + \\ &\quad \frac{\pi\alpha_n\mu\rho g}{6m} z d_1\left[3{d_1}^2 + 3d_1(R-z) - 2z(3R-z)\right]. \end{aligned} \tag{30}$$

To find the penetration depth, this may be solved numerically for the depth at which the velocity vanishes.

# References


[1] T. A. Brzinski III and D. J. Durian, "Characterization of the drag force in an air-moderated granular bed", Soft Matter **6**, 3038-43 (2010).

[2] K. Wieghardt, "Experiments in Granular Flow", Annu. Rev. Fluid Mech. **7**, 89 (1975).

[3] R. Albert, M. A. Pfeifer, A. L. Barabási, and P. Schiffer, "Slow drag in a granular medium", Phys. Rev. Lett. **82**, 205 (1999).

[4] D. J. Costantino, J. Bartell, K. Scheidler, and P. Schiffer, "Low-velocity granular drag in reduced gravity", Phys. Rev. E **83**, 011305 (2011).

[5] H. Katsuragi, and D. J. Durian, "Unified force law for granular impact cratering", Nature Physics **3**, 420-3 (2007).

[6] M. A. Ambroso, R. D. Kamien, and D. J. Durian, "Dynamics of shallow impact cratering", Phys. Rev. E **72**, 041305 (2005).

# Part II: Experiment


## Abstract

Here we expand upon our discussion of the experimental results presented in the main text. In the first section we focus on the results for the quasi-static lowering of cylinders and cones. We explicitly contrast these results with the expectation for a stopping force oriented parallel to the projectile surface. We also revisit the airflow-dependence of the force, and present further analysis which reiterates the results presented in the main text: the force is linear in air-speed, and vanishes at a value independent of depth indicating that gravity loading, not motion-loading, sets the frictional force. Then we investigate the stick-slip fluctuations common in all quasi-static lowering experiments, as mentioned in the main text. The second section describes follow-up experiments in which we measure the resisting force experienced by slowly, continuously lowered intruders. Surprisingly, we find different behavior than that observed for the quasistatically lowered intruders that were the focus of the main text.


# 1 Quasi-static lowering of cylinders and cones

## 1.1 Further evidence against a surface-tangent force

In the main text, we argue that the force acting on an intruder lowered quasi-statically onto a granular packing is oriented exactly normal to the intruder surface. This conclusion was supported by experimental measurements of the quasi-static resisting force, $F(z)$, that exhibit the depth- and geometry-dependence consistent with this assumption. For completeness, we now present further evidence that excludes the opposite limit.

The surface-tangential prediction for the stopping force, as calculated in Supplemental Material, Part I, is

$$\frac{F(z)}{\alpha_t \mu \rho g} = \begin{cases} \pi R z^2 & \text{cylinder} \quad (1a) \\ (\pi/3) \tan\phi \ z^3 & \text{cone} \quad (1b) \end{cases}$$

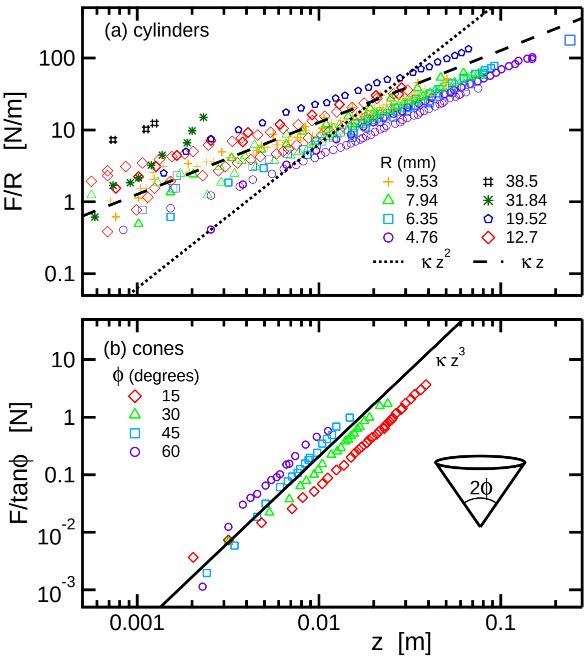


Figure 1: The rate-independent component of the drag, $F(z)$, for (a) cylindrical probes normalized by radius $R$ with the dependence on depth, $z$, expected for d$\mathbf{F}$ parallel (perpendicular) to the projectile surface plotted as a dotted (dashed) line; (b) conical probes normalized by the tangent of the apex half-angle, $\tan\phi$, plotted against $z$, with the expected depth scaling, $\kappa z^3$, plotted as a solid line.

Where $z$ is the instantaneous depth, $\mu$ is an internal friction coefficient equal to the tangent of the repose angle, $\rho g$ is the effective gravitational pressure gradient, and $\alpha_t$ is a dimensionless proportionality constant. As shown in Supplemental Material, Part I, the projectile-geometry dependence is quite different under the assumption that the force is oriented surface-normal. For cylinders, it would scale as $R^2 z$ rather than $Rz^2$ and for cones it would scale as $\tan^2\phi$ rather than $\tan\phi$. Thus we plot (a) $F(z)/R$ vs $z$ for cylinders, and (b) $F(z)/\tan\phi$ vs $z$ for cones. In sharp contrast with the normalization presented in the main text, this fails to collapse the data. Even if, by some serendipity, this treatment were to collapse the data, there remains the issue of the depth-dependence. For the case of cones, drag both normal and tangential to the surface are proportional to $z^3$. However, for cylinders, the depth dependence is linear for surface-normal drag and quadratic for surface-tangential drag. These two proportionalities are plotted in Fig. 1(a) as dashed and dotted lines, respectively. Again, the data fail to agree with the tangential-force prediction. In contrast, the agreement with the normal-force prediction is excellent.

## 1.2 Further evidence for gravity-loading of frictional contacts

The force opposing the motion of a quasistatically lowered projectile must be the consequence of friction at contacts that are loaded either by gravity or by the motion of the projectile. While the gravity-loading of the packing is modified by a sub-fluidizing upflow of air, the motion loading is not. The reduction in the gravitational pressure gradient due to an upflow of air is known to scale as $1-U/U_c$, where $U$ is the superficial air-speed through the bed, and $U_c$ is the critical air-speed at which the granular material is fluidized [1, 2]. In the main text, we demonstrate that data for force plotted against depth for many airflows collapse when normalized by $1-U/U_c$. This approach enables us to quickly illustrate the role of gravity-loading within the bed for all geometries tested, but the same physics may be more explicitly demonstrated as in Fig. 2. Here the force acting on a sphere is normalized by the depth, and plotted against the air-speed of the applied upflow of air. We see the exact behavior expected for a drag force set by the gravity-loading of the bed: the force is linear with air-speed, and goes to zero at the same air-speed for all depths (indicated by color and symbol). The linear fit to $F(z)/z$ versus $U$ vanishes at $U_c = 0.087 \pm 0.004$ m/s, which is in good agreement with the observed onset of bubbling at $U = 0.089 \pm 0.002$ m/s.

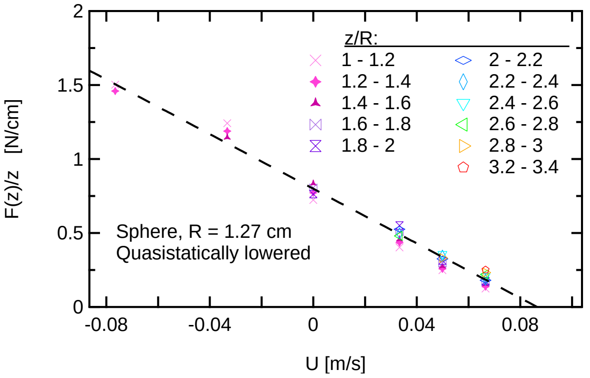


Figure 2: The force exerted by a granular packing upon a quasistatically lowered sphere, divided by the depth, and plotted against the superficial air-speed. All data are for a sphere 1.27 cm in radius. For spheres, the $1/z$ normalization is approximately valid only for $z > R$, so we plot data for several values of $z/R > 1$ as indicated by Symbol and color. The dashed line is a linear fit.

## 1.3 Stick-slip behavior for quasistatically lowered intruders

Next we describe the intermitent quality of the projectile motion during our quasistatic lowering experiments. Specifically, below a short initial penetration depth we observe stick-slip behavior: the penetration depth remains constant while the load on the granular media increases. Once the load reaches some critical value, the granular material fails, and the projectile falls a short distance, coming to rest at a new depth. In the

main text, our interest is in the conditions for flow, so only the peaks of these fluctuations are considered, but here we consider the fluctuations themselves. Measurements of $F(z)$ for which these fluctuations have *not* been processed out, and which are normalized according to Eq. (3) in the main text, are plotted against $z$ in Fig. 3. Such fluctuations are common in a range of friction dominated systems, and an extensive study of the stick-slip behavior in our system would merit a paper of its own. In Ref. [3], the authors undertake a study of stick-slip motion for slow, horizontal motion through a granular bed, where the mechanics ought to be similar to our system. They show that, in the absence of system size effects, the magnitude of the fluctuations are proportional to the average drag force. It is pertinent to note that stick-slip behavior generically depends on the intruder mass and the spring constant of the force gauge, as well as the properties of the granular medium. For the data presented in Fig. 3(a) the cylindrical intruders all have a mass of 0.5 kg, and the force gauge has a spring constant of 40.5 N/m. In Fig. 3(b) the conical intruders all have a mass of 0.1 kg, and the force gauge has a spring constant of 16.2 N/m. We have not systematically varied any of these quantities.

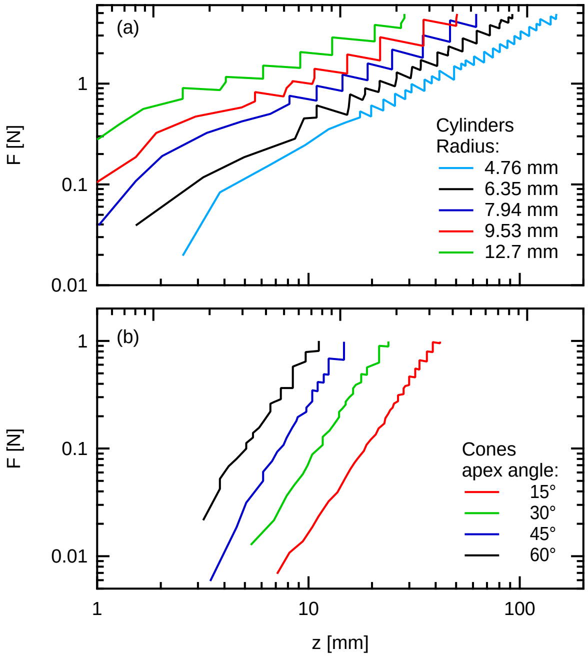


Figure 3: The rate-independent component of the stopping force, $F(z)$, both for (a) cylinders and (b) cones, plotted against depth $z$ where the stick-slip fluctuations haven't been removed. The sawtooth structure here is characteristic of all data discussed in the main text.

For cylinders, as shown in Fig. 3(a), the onset of stick-slip motion occurs at a force of roughly 0.5 N for all radii. Above this threshold, we see the same thing as in Ref. [3]: the fluctuations are always close to 20% of the magnitude of the force, independent of intruder geometry or depth. For cones, the story is slightly different. The onset of stick-slip is smaller, at a force of roughly 0.2 N for all apex angles, and the magnitude of the fluctuations grows with depth. This may be a consequence of the depth-dependence of the cross-section of the cones, but the fluctuations are on the order of 10% for the full dynamic range measured in the present work.

# 2 Resistance to slow, *continuous* motion

For slow, quasistatic lowering of intruders onto granular packings we observe pronounced stick-slip motion, and find that the magnitude of the resisting force is dependent on the gravity-loading of the bed rather than the motion-loading. The situation could conceivably be different for slow continuous motion at $v \neq 0$, where the grains are being continuously motion-loaded, and where stick-slip fluctuations cannot relax the packing. We test this by attaching an intruder to the crossarm of an Instron model 5564 table-mounted Materials Testing System (MTS), and driving our cylindrical and conical intruders into packings of the same grains as used in the main text. The MTS enables us to drive the intruder at a constant rate, and simultaneously measure the force acting on the intruder.

Measurements of $F(z)$ for cylinders lowered in this manner at a rate of 4 mm/min are normalized by $\pi R^2$, according to the surface-normal expectation, and plotted against $z$ in Fig. 4(a). Here we also provide measurements of $F(z)$ from quasi-static lowering for comparison. We observe that, for small $z$, the drag is the same for both quasistatic and continuous lowering. But for depths greater than 1 cm the force acting on a cylinder is larger for continuous motion, with a depth dependence approaching $z^2$ at greater depths. This is consistent with an additive mixing of surface-normal and -tangential stopping forces of the form

$$\frac{F(z)}{\mu\rho g} = \begin{cases} \pi R\left(\alpha_t z^2 + \alpha_n R z\right) & \text{cylinder} \quad (2a) \\ (\pi/3)\left(\alpha_t \tan\phi + \alpha_n \tan^2\phi\right) z^3 & \text{cone} \quad (2b) \end{cases}$$

For our packings, we measure the internal coefficient of friction, $\mu = 0.4$, and the bulk granular density, $\rho = 1.48$ g/cm$^3$. With these numbers, the data are fit well using coefficients $\alpha_n = 70$ and $\alpha_t = 11$ for the normal and tangential force laws respectively.

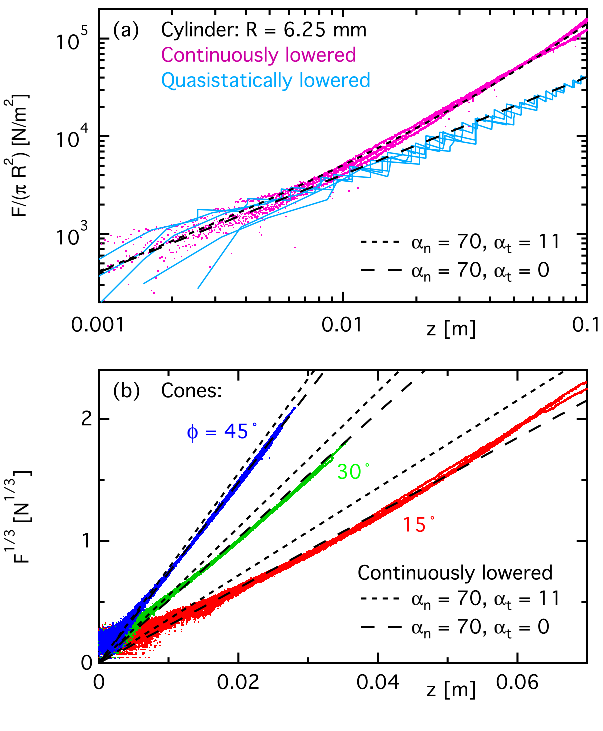


Figure 4: (a) $F(z)$ for a 6.35 mm radius cylinder continuously lowered at a rate of 4.0 mm/min (magenta points), or lowered quasistatically as described in the main text (cyan line segments), normalized by $\pi R^2$ in order to collapse the data according to the prediction for a force acting normal to the projectile surface as described in Supplemental Material, Part I. (b) $F(z)$ for cones continuously lowered at a rate of 4.0 mm/min, normalized by $\tan^2 \phi$ in order to collapse the data according to a the prediction for a force acting normal to the projectile surface as described in the main text. In (a) and (b), Eq. (2) is plotted as dashed lines where $\alpha_n = 70$ and $\alpha_t = 0$ for the short-dashed line, and $\alpha_n = 70$ and $\alpha_t = 11$ for the long-dashed line.

Perhaps the constant motion prevents grains adjacent to vertical face of the intruder from relaxing into stable configurations, resulting in an enriched population of contact forces which can only contribute to the total force by means of sliding friction at the intruder surface.

Measurements of $F(z)$ for cones lowered in the same fashion are linearized by taking the cube root, and plotted against $z$ in Fig. 4(b). Unlike the case of cylinders, the force acting on a cone lowered at a constant speed is consistent with a purely surface-normal orientation, though the magnitude of $\alpha_n$ is double that observed for quasistatic lowering, as described in the main text. Interestingly, this means that continuously lowered cones experience the same $\alpha_n$ as cylinders lowered quasi-statically at $U = 0$. This result is surprising, especially given our success in describing data from actual impacts using the value $\alpha_n = 35$.

While the data for continuously lowered cones agree well with the model presented in the main text, close inspection of Fig. 4(b) reveals that taking the cube root of the force does not perfectly linearize the data. Instead, for all three apex angles, the data exhibit a weak, upward curvature. This may be the consequence of sand, displaced by the motion of the intruder, mounding at the packing surface near the intruder, thus effectively increasing the depth of penetration. While the results presented in the main text seem to describe the general behavior of intruders undergoing constant motion, second-order effects such as this may become more important when the motion is continuous.

# References


[1] D. Geldart, *Gas Fluidization Technology*, (Wiley, London, 1986).

[2] D. Gidaspow, *Multiphase flow and fluidization*, (Academic, Boston, 1994).

[3] I. Albert, P. Tegzes, R. Albert, J. G. Sample, A.-L. Barabási, T. Vicsek, B. Kahng and P. Schiffer, "Stick-slip fluctuations in granular drag", Phys. Rev. E **64**, 031307 (2001).
